# Supplementary material for: Zero NeRF: Registration with Zero Overlap
Source: arXiv:2211.12544 source file (2022-11-22)
Supplement: Supplementary file 1 [file 7_appendix.tex]

\appendix
\section{Full Results}

% \section{Implementation Details}
